# Supplementary material for: Strategize Before Teaching: A Conversational Tutoring System with Pedagogy Self-Distillation
Source: arXiv:2302.13496 source file (2023-02-27)
Supplement: Supplementary file 1 [file appendix.tex]

\clearpage
\appendix
\section*{Appendix}
\section{Datasets and Parameter Setting}
\label{sec:appendix:data_para}
\paragraph{Datasets.}
\begin{table}[t]
\setlength{\tabcolsep}{1mm}\small
\begin{center}
% \resizebox{\linewidth}{!}{
\begin{tabular}{l|ccc}
\toprule[1.0pt]
& \textbf{CIMA}  &\textbf{TSCC}  &\textbf{TalkMoves}\\
\midrule[0.5pt]
Setting &role play &one to one & transcript \\
Knowledge & Italian &English &Math \\
\# of Instances &3,315 &4,337 &9,998 \\
\# of Teaching Strategies &5 &21 &6 \\
\midrule[0.5pt]
% \# of instances &  &  \\
avg length of source &45.6 &687 &42.2 \\
avg length of target &9.7 &13.4 &8.9 \\

\bottomrule[1.0pt]
\end{tabular}
\end{center}
\vskip -0.5em
\caption{\label{tab:data_statistic} Statistics of CIMA, TSCC and TalkMoves.
}
\vskip -0.5em
\end{table}
\begin{table}[t]
\setlength{\tabcolsep}{1mm}\small
\begin{center}
\begin{tabular}{lp{5.8cm}}
\toprule[1.0pt]
\textbf{Dataset}  & \textbf{Teaching Strategy}\\
\midrule[0.5pt]
\textbf{CIMA} &  Hint/Information Reveal, Question, Confirmation, Correction, Other \\
\midrule
\textbf{TSCC} & Opening, Topic opening, Development, Eliciting, NA, Scaffolding, Exercise, Enquiry, Repair, Closing, Presentation, Clarification, Homework, Recap, Disruption, Topic closure, Redirecting, Revision, Topic initiation, Admin, Reference\\
\midrule
\textbf{TalkMoves} & Press for accuracy, Getting to relate, Revoicing, Keeping everyone together, Press students for reasoning, Restating\\
\bottomrule[1.0pt]
\end{tabular}
\end{center}
\vskip -0.5em
\caption{\label{tab:DA_list} Teaching strategy lists.
}
\vskip -1.5em
\end{table}
\begin{figure}[t]
\centering
\subfigure[CIMA]{\label{sfig:cima_fre}
\includegraphics[width=0.39375\linewidth]{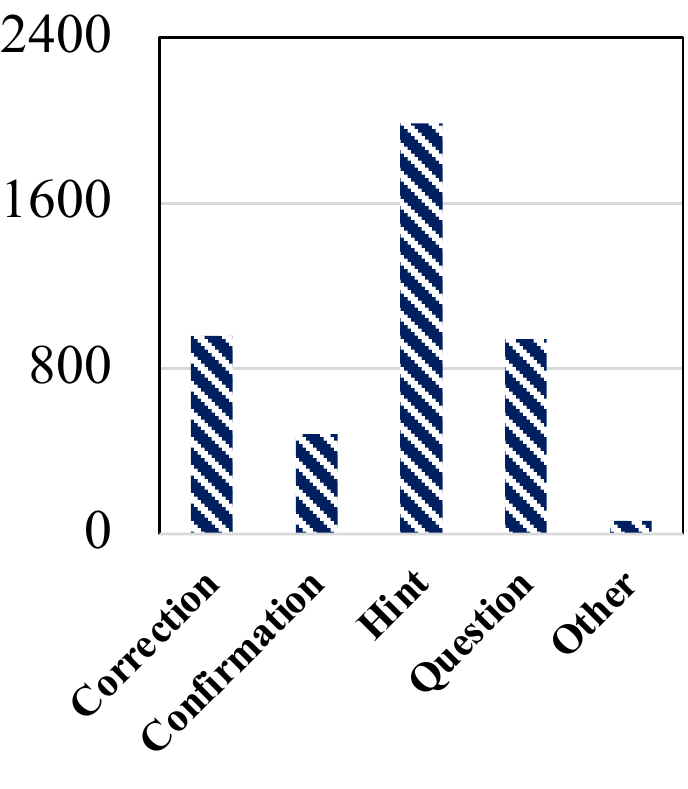}
}
\subfigure[TalkMoves] {\label{sfig:talk_fre}
\includegraphics[width=0.50625\linewidth]{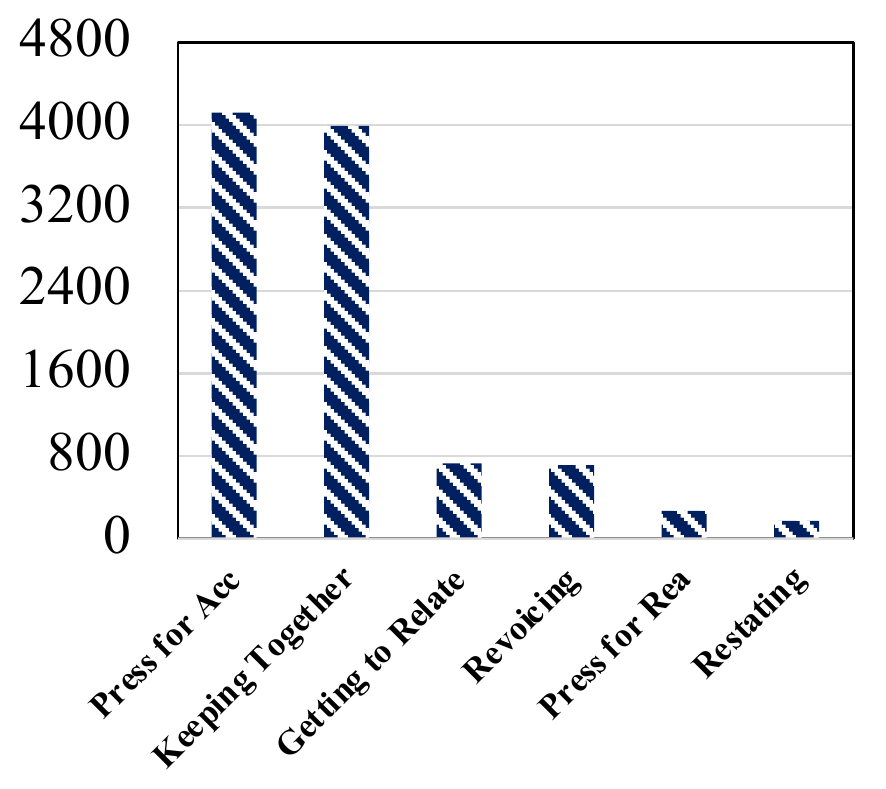}
}
\vskip -0.5em
\subfigure[TSCC] {\label{sfig:tscc_fre}
\includegraphics[width=0.9\linewidth]{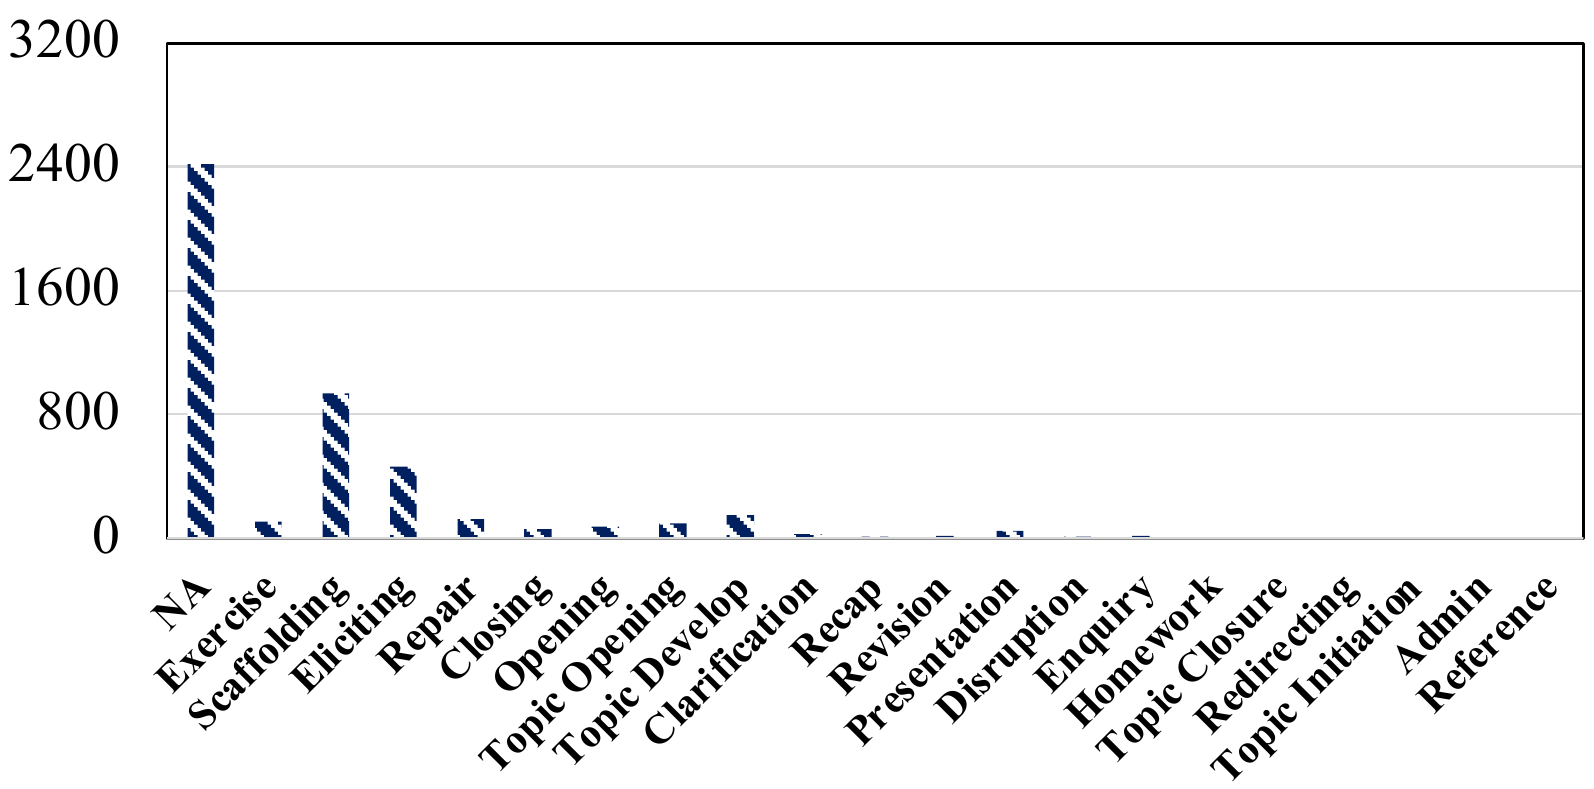}
}
\vskip -1em
\caption{\label{fig:da_fre}Frequency over teaching strategy . 
}
\vskip -0.5em
\end{figure}
We use three datasets to do the experiments. They are CIMA \cite{stasaski-etal-2020-cima}, TSCC \cite{caines2020teacher} and TalkMoves \cite{suresh2019automating,suresh2022talkmoves}. CIMA contains one-to-one conversations that focus on teaching students to translate a phrase from English to Italian. TSCC focuses on teaching English for eight non-native English-speaking students. TalkMoves is constructed by transcripts of math classrooms. The statistics of the three datasets are shown in Table \ref{tab:data_statistic}. We can find that the three datasets are quite small and the number of instances are all less then 10,000. 

We also list the teaching strategies of the three datasets in Table \ref{tab:DA_list} and the frequency distribution of them in Figure \ref{fig:da_fre}. We can find that the data imbalance problem of the datasets is severe. 

\paragraph{Parameter Settings.}
We use BART-Base\footnote{\url{https://github.com/facebookresearch/fairseq/tree/main/examples/bart}} and mBART-Large\footnote{\url{https://github.com/facebookresearch/fairseq/tree/main/examples/mbart}} models to initialize our model, respectively. 
BART-Base model has $6$ layers of encoder and decoder with $768$ hidden dimension, while mBART-Large has $12$ layers of encoder and decoder with $1024$ hidden dimension. The parameter sizes for the two models initialized with BART and mBART are 199M and 816M, respectively.

We use one NVIDIA RTX 3090 GPU to train our model.
During training, we set the max tokens of each batch to 1024 (for BART, or 512 for mBART) with an update frequency of 4. We adopt Adam optimizer~\cite{kingma:adam} with learning rate selected in $\{$1e-4, 5e-5, 2e-5, 1e-5$\}$
and warm-up updates selected in $\{$200, 500, 1000$\}$ followed by a polynomial decay scheduler.
Dropout strategy~\cite{Srivastava:2014:DSW:2627435.2670313} with dropout rate selected in $\{$0.2, 0.4$\}$ and $L_2$ regularization with 0.01 effect value, as well as early stoping based on validation performance, are used to alleviate overfitting.
We set the tradeoff values among the losses as $\lambda=1.0$, $\gamma=1.0$ and $\delta=0.2$.
The training cost is listed in Table~\ref{tab:train_time}.
During inference, predicting threshold $\theta=0.3$ and beam size is set to 5.

\begin{table}[t]
\setlength{\tabcolsep}{1.7mm}\small
\begin{center}
\newcommand{\tabincell}[2]{\begin{tabular}{@{}#1@{}}#2\end{tabular}}
\begin{tabular}{lcccc}
\toprule[1.0pt]
\multirow{2}{*}{\textbf{Dataset}}  & \multicolumn{2}{c}{ \tabincell{c}{\textbf{Train Time/Epoch}}} & \multicolumn{2}{c}{ \tabincell{c}{\textbf{Train Epochs}}}\\
\cmidrule(lr){2-3}\cmidrule(lr){4-5}
& BART & mBART & BART & mBART \\
\midrule[0.5pt]
\textbf{CIMA} & 0.5 min & 2 min & 11 & 33 \\
\textbf{TSCC} & 4.5 min & 10 min & 18 & 32\\
\textbf{TalkMoves} & 1 min & 6 min & 32 & 65 \\
\bottomrule[1.0pt]
\end{tabular}
\end{center}
\vskip -0.5em
\caption{\label{tab:train_time} Training time per epoch and training epoch numbers for the three datasets.
}
\vskip -0.5em
\end{table}

\section{Details of Baselines and Evaluation}
\paragraph{Baselines.} We introduce BiLSTM, Transformer in Table \ref{tab:main_gen} here. (i) BiLSTM: It's based on a 1 layer BiLSTM encoder and 1 layer BiLSTM decoder with a 512 hidden size. (ii) Transformer: It's based on 6 layers of Transformer encoder and 6 layers of Transformer decoder with a 512 hidden size. 

\paragraph{Evaluation Setting.} $\dagger$ in Table \ref{tab:ts_prediction} indicates the prediction is based on the target tutor response, i.e., we use $\bm{h}_t^{\langle \text{eos}\rangle}$ (see Section~\ref{sec:model:cts}) to do the teaching strategy prediction, while the rest results all use $\bm{h}_s^{\langle \text{eos}\rangle}$ for prediction. 

The three evaluation settings in Table \ref{tab:main_gen} imply three levels of generation difficulties. ``W/O TS'' means no teaching strategy in both training and testing, which generates responses only based on context. ``With Golden TS'' means using ground-truth teaching strategy to guide the generation in both training and testing. ``Need TS Prediction'' means ground-truth teaching strategy labels only used in training but we need to predict the strategy before generation in testing.
