# Supplementary material for: Strategize Before Teaching: A Conversational Tutoring System with Pedagogy Self-Distillation
Source: arXiv:2302.13496 source file (2023-02-27)
Supplement: Supplementary file 2 [file appendix_DAfre.tex]

\begin{figure}[t]
\centering
\subfigure[CIMA]{\label{sfig:cima_fre}
\includegraphics[width=0.39375\linewidth]{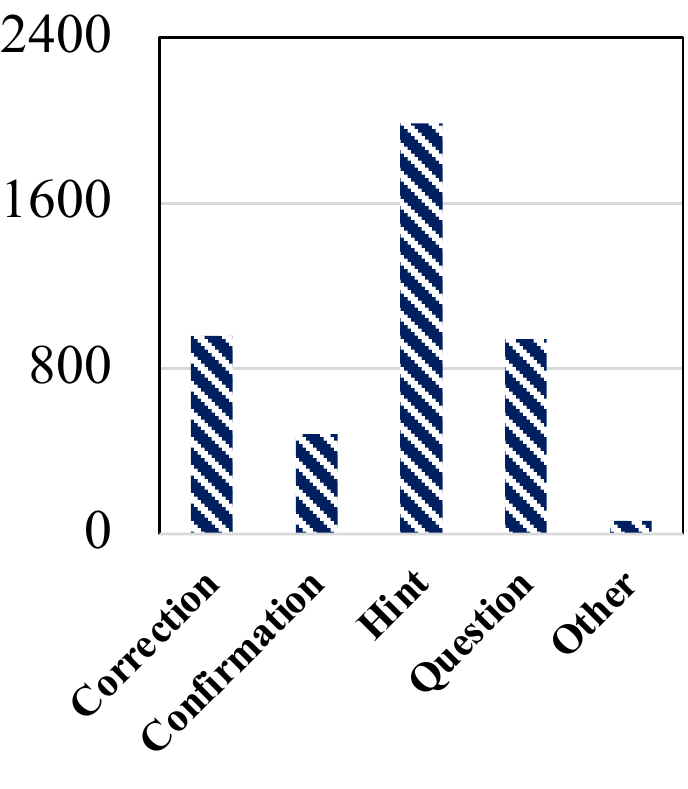}
}
\subfigure[TalkMoves] {\label{sfig:talk_fre}
\includegraphics[width=0.50625\linewidth]{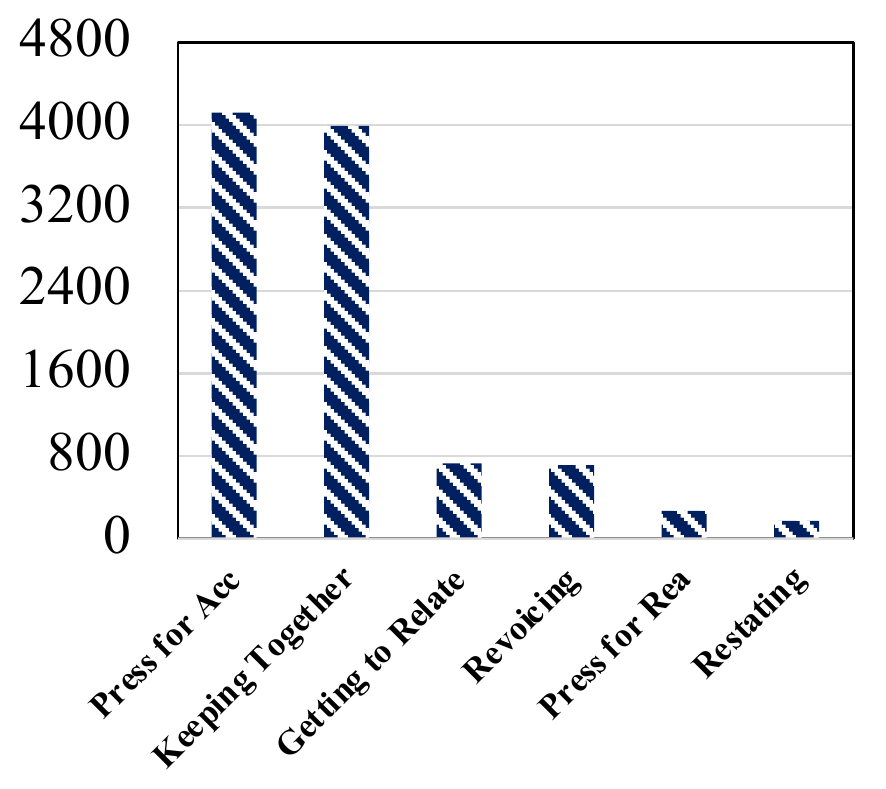}
}
\vskip -0.5em
\subfigure[TSCC] {\label{sfig:tscc_fre}
\includegraphics[width=0.9\linewidth]{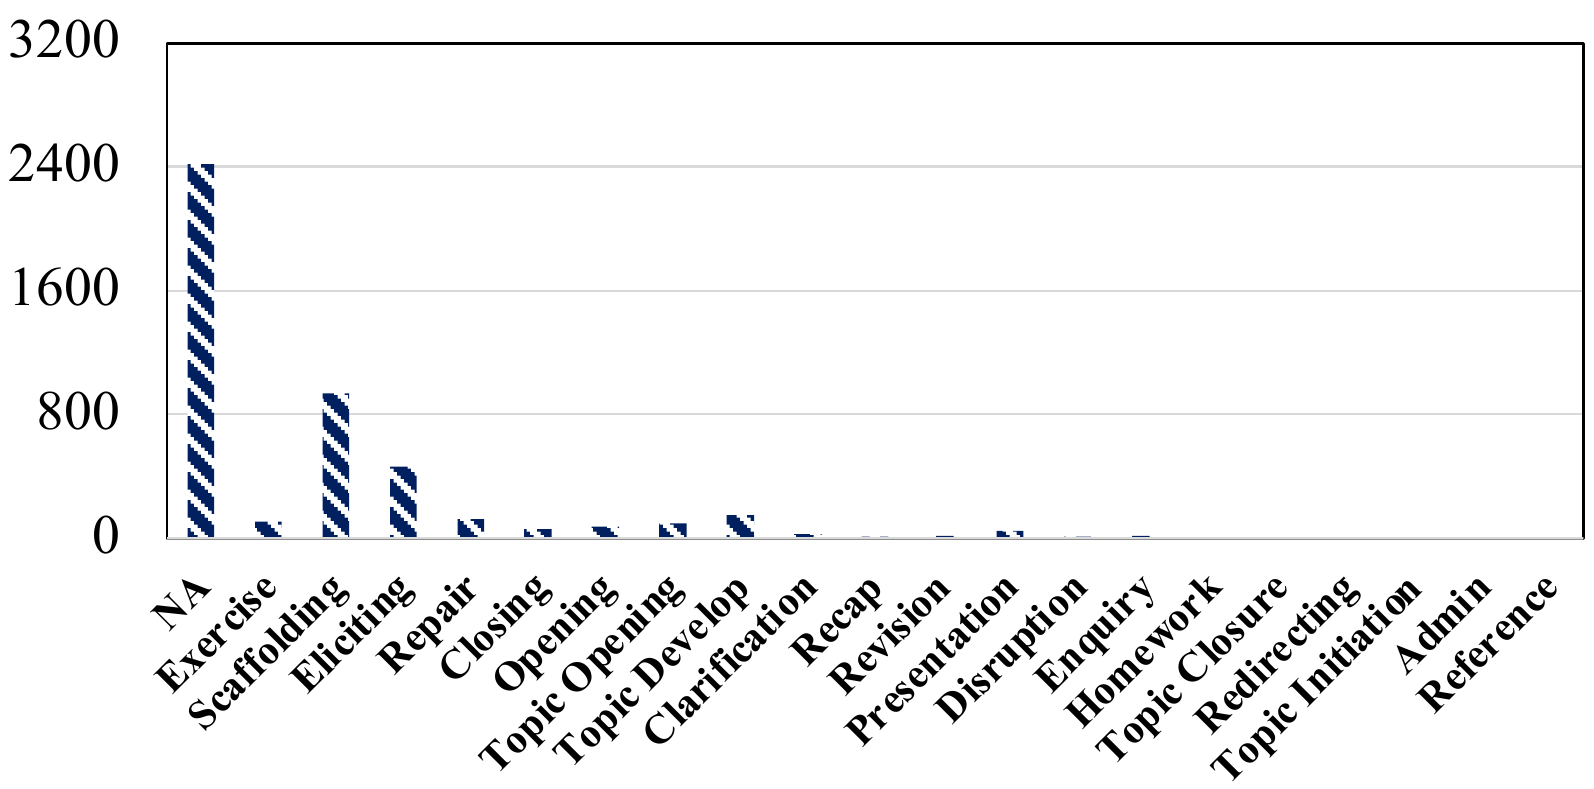}
}
\vskip -1em
\caption{\label{fig:da_fre}Frequency over teaching strategy . 
}
\vskip -0.5em
\end{figure}
