# Supplementary material for: Strategize Before Teaching: A Conversational Tutoring System with Pedagogy Self-Distillation
Source: arXiv:2302.13496 source file (2023-02-27)
Supplement: Supplementary file 3 [file appendix_DA_list.tex]

\begin{table}[t]
\setlength{\tabcolsep}{1mm}\small
\begin{center}
\begin{tabular}{lp{5.8cm}}
\toprule[1.0pt]
\textbf{Dataset}  & \textbf{Teaching Strategy}\\
\midrule[0.5pt]
\textbf{CIMA} &  Hint/Information Reveal, Question, Confirmation, Correction, Other \\
\midrule
\textbf{TSCC} & Opening, Topic opening, Development, Eliciting, NA, Scaffolding, Exercise, Enquiry, Repair, Closing, Presentation, Clarification, Homework, Recap, Disruption, Topic closure, Redirecting, Revision, Topic initiation, Admin, Reference\\
\midrule
\textbf{TalkMoves} & Press for accuracy, Getting to relate, Revoicing, Keeping everyone together, Press students for reasoning, Restating\\
\bottomrule[1.0pt]
\end{tabular}
\end{center}
\vskip -0.5em
\caption{\label{tab:DA_list} Teaching strategy lists.
}
\vskip -1.5em
\end{table}
