# Supplementary material for: Strategize Before Teaching: A Conversational Tutoring System with Pedagogy Self-Distillation
Source: arXiv:2302.13496 source file (2023-02-27)
Supplement: Supplementary file 4 [file appendix_train_time.tex]

\begin{table}[t]
\setlength{\tabcolsep}{1.7mm}\small
\begin{center}
\newcommand{\tabincell}[2]{\begin{tabular}{@{}#1@{}}#2\end{tabular}}
\begin{tabular}{lcccc}
\toprule[1.0pt]
\multirow{2}{*}{\textbf{Dataset}}  & \multicolumn{2}{c}{ \tabincell{c}{\textbf{Train Time/Epoch}}} & \multicolumn{2}{c}{ \tabincell{c}{\textbf{Train Epochs}}}\\
\cmidrule(lr){2-3}\cmidrule(lr){4-5}
& BART & mBART & BART & mBART \\
\midrule[0.5pt]
\textbf{CIMA} & 0.5 min & 2 min & 11 & 33 \\
\textbf{TSCC} & 4.5 min & 10 min & 18 & 32\\
\textbf{TalkMoves} & 1 min & 6 min & 32 & 65 \\
\bottomrule[1.0pt]
\end{tabular}
\end{center}
\vskip -0.5em
\caption{\label{tab:train_time} Training time per epoch and training epoch numbers for the three datasets.
}
\vskip -0.5em
\end{table}
